# Supplementary material for: Active tuning of synaptic patterns enhances immune discrimination
Source: arXiv:1810.06015 source file (2018-10-14)
Supplement: Supplementary file 1 [file ms_SI.pdf]

# Supplementary Information: Active tuning of synaptic patterns enhances immune discrimination

Miloš Knežević and Shenshen Wang
*Department of Physics and Astronomy, University of California Los Angeles, Los Angeles, CA 90095, USA*
(Dated: October 14, 2018)

## I. DETAILS OF THE MODEL

### Initial and boundary conditions

The membrane separation is fixed at $l_i = 100\,\text{nm}$ at and outside the boundary of the contact zone, i.e., $r \geq r_1$. Initially, the B-cell membrane profile is described by $l(r) = l_0 + cr^4$; here $l_0 = 45\,\text{nm}$, and a constant $c > 0$ is chosen such that the boundary condition at $r = r_1$ is satisfied. The boundary of the simulation domain $r = r_2$ is non-permeable for all proteins. We draw initial positions $(x, y)$ of all types of proteins from a 2D uniform distribution in $[0, L] \times [0, L]$, where $L$ is the linear dimension of the lattice.

### Discretized operators

The Laplacian $\Delta_d l(x, y)$ and gradient $\nabla_d l(x, y)$ operators take a discretized form: $\Delta_d l_i \equiv \Delta_d l(x, y) = l(x+a, y) + l(x-a, y) + l(x, y+a) + l(x, y-a) - 4l(x, y)$, and $(\nabla_d l_i)^2 \equiv [\nabla_d l(x, y)]^2 = [l(x+a, y) - l(x, y)]^2 + [l(x, y+a) - l(x, y)]^2$, where $(x, y)$ denote the Cartesian coordinates of a lattice site $i$.

### Force

In our current model, we consider normal forces that pull on sufficiently large clusters of bound BCR-Ag pairs with a constant magnitude per bond. In other words, the total magnitude of pulling force on an above-threshold cluster scales with the cluster size. This choice of force application scheme is motivated by B cell biology: The pulling forces exerted by B cells originate from the contractile forces generated by myosin II motor proteins on the cortical F-actin cytoskeleton, which has BCRs attached. Quantification of the actomyosin localization in the B-cell synapses indicates that the amount of myosin II and F-actin correlates with the size of antigen microclusters [1]. In addition, direct activation of myosin II by the BCR has been described [2], suggesting that BCR signaling control the timing and intensity of myosin contractility. Taken together, it is conceivable that the feedback between the degree of receptor clustering that triggers BCR signaling and the strength of pulling in response to signaling gives rise to positive correlations between force and cluster size.

### Monte Carlo propagation

In each Monte Carlo (MC) step, we attempt membrane moves (change of local membrane separation $l_i$) and protein hopping moves (change of protein occupation numbers $n_i$). First, for membrane patches $i$ that do not belong to any of the clusters $C_j$ bigger than $n_t$, we attempt to change locally the distance $l_i$ between the membranes, by a displacement $\Delta l_i = l\zeta$, where $l = 10\,\text{nm}$ is the displacement width, and $\zeta$ is a random number drawn from a uniform distribution between $[-1, 1]$. Membrane displacements that would lead to $l_i + \Delta l_i < 0$ are rejected. For displacements that satisfy $l_i + \Delta l_i \geq 0$, we calculate the change in configurational energy $\Delta H$ between the new and current configurations, and decide whether to accept the MC move according to Metropolis-Hastings criterion. In contrast, to model mechanical pulling, for all the patches $i$ within a cluster $C_j$ we draw a single displacement $\Delta l_j = l\tilde{\zeta}$ and attempt to apply it to the cluster as a whole. In this case, the random number $\tilde{\zeta}$ is drawn from the interval [0,1], as it is very unlikely to have a smaller separation between membranes while a pulling force is exerted to disrupt a cluster of bound receptors and ligands. If a displacement $\Delta l_j$ is such that less than 80% of patches within a cluster would have $l_i + \Delta l_j$ that fall outside of the binding range for BCR-Ag molecules, the MC move is rejected. Otherwise, the move is accepted according to the Metropolis-Hastings criterion, and an entire cluster of bonds is ruptured.

During a MC step, we also attempt diffusive moves of all types of proteins present in the model. This motion is modelled as a hopping process between nearest-neighbor membrane patches. Only within the contact region ($r \leq r_1$) may an attempted hopping of a protein change the configurational energy, while hopping events in the non-interacting region ($r_1 < r \leq r_2$) have no energetic effect. The proteins are however free to move between the two regions, and the non-interacting zone thus acts as a reservoir of free protein molecules.

### Time scale

We construct a rough estimate of the timescale associated with one MC step. For the chosen membrane patch length scale $a = 70\,\text{nm}$, diffusive motion of proteins is typically slower than membrane relaxation, and thus sets

the timescale. The typical diffusion constant for proteins tethered to a membrane is $D \simeq 1\,\mu\mathrm{m}^2/\mathrm{s}$, and hence one MC step corresponds to $t = a^2/4D \simeq 1\,\mathrm{ms}$ of real time.

## II. PULLING-INDUCED SHIFT OF THE COARSENING TRANSITION

As seen in Fig. 2 (main text), the initial departure of a discrimination curve from the approximate plateau (i.e., leaving regime II of arrested phase separation) signals the onset of the coarsening transition (i.e., entering regime III of structural percolation). The transition point marks the minimal binding affinity that is just sufficient to overcome the pulling force, thus allowing BCR-bound Ag clusters to grow beyond the threshold size. Interestingly, as the pulling force strengthens, the transition point shifts to higher affinities in a nearly linear manner; as $Fl$ increases from 14 to 22 to $30\,k_BT$, the corresponding transition affinity, $U^*_{BA}$, rises from 7 to 11 to $15\,k_BT$. Below we present a phenomenological model that captures this linear dependence under strong pulling forces.

Near but below the coarsening transition, receptor clusters remain well-separated and have similar local environments. Thus, consider a *typical* cluster that is held close to the threshold size under pulling. At the onset of cluster growth, when BCR-Ag binding affinity slightly exceeds $U^*_{BA}$, the growth rate is small compared to the force-free unbinding rate; the system would reach a quasi-steady state described by the dynamic balance between unbinding and rebinding events:

$$\frac{N_b(t)}{DC_\infty t - N_b(t)} \simeq e^{\beta[U_{BA} - f(t) l_b / N_b(t)]}. \tag{1}$$

Here $DC_\infty$ denotes a constant influx of free pairs of Ag and BCRs into the contact zone; free molecules are maintained at a concentration $C_\infty$ in the reservoir (the non-adhering region of apposing membranes) and diffusing with a uniform diffusivity $D$. At a given time $t$, out of a supply of $DC_\infty t$ molecules, a number $N_b(t)$ are bound and a number $DC_\infty t - N_b(t)$ are unbound. A linearly ramping *total* force during cluster growth, $f(t) = \dot{f}\,t$, distributes evenly among the $N_b(t)$ bound molecules. Force acts along a reaction coordinate, reaching $l_b$ at the transition state barrier between bound and unbound states; $\beta^{-1} = k_BT$ sets the energy scale.

We are interested in a solution of the form $N_b(t) = \dot{N}_b\,t$, then Eq. 1 becomes a relation between the rates:

$$\frac{\dot{N}_b}{DC_\infty - \dot{N}_b} = e^{\beta[U_{BA} - \dot{f} l_b / \dot{N}_b]}. \tag{2}$$

At a given loading rate $\dot{f}$, a steady growth solution ($\dot{N}_b > 0$) first appears at the critical binding affinity, $U^*_{BA}$. Introducing dimensionless cluster growth rate $x = \dot{N}_b / DC_\infty$ and loading rate $\alpha_f = \beta \dot{f} l_b / DC_\infty$, we obtain

$$\frac{x}{1-x} = e^{\beta U_{BA} - \alpha_f / x}. \tag{3}$$

To determine the minimal affinity $U^*_{BA}$ that supports a solution $x \in (0,1)$, we perform a bifurcation analysis of the quasi-steady state behavior (Eq. 3); a saddle-node bifurcation occurs when $g(x) \equiv x/(1-x)$ and $h(x) \equiv \exp(\beta U_{BA} - \alpha_f/x)$ are tangential at the point $x^*$ where they touch, i.e., $g(x^*) = h(x^*)$ and $g'(x^*) = h'(x^*)$. These lead to

$$\frac{\alpha_f}{x^*} = \frac{1}{1-x^*} > 1, \tag{4}$$

and

$$\frac{\alpha_f}{x^*} - 1 = e^{\beta U^*_{BA} - \alpha_f / x^*}. \tag{5}$$

Eq. 5 relates the transition affinity to the loading rate:

$$\beta U^*_{BA} = \frac{\alpha_f}{x^*} + \log\left(\frac{\alpha_f}{x^*} - 1\right), \tag{6}$$

where $\alpha_f / x^* = \beta \dot{f} l_b / \dot{N}^*_b$. Therefore, under high loading rates (hence large $\alpha_f / x^*$), the linear term in Eq. 6 dominates, and we arrive at

$$\beta U^*_{BA} \simeq \beta \dot{f} l_b / \dot{N}^*_b. \tag{7}$$

Recognizing that $\dot{f}/\dot{N}^*_b$ corresponds to the magnitude of normal force $F$ pulling on each *single* BCR-Ag bond in an above-threshold cluster (Eq. 4, main text), Eq. 7 predicts a linear shift in the coarsening transition with strengthening pulling force, as confirmed by simulations.

## III. ALTERNATIVE FORCE APPLICATION SCHEMES

The affinity discrimination curves relate the total amount of BCR-Ag binding to the timing and magnitude of pulling forces: the height and width of the plateau, which spans the intermediate-affinity regime and signifies arrested phase separation, are *respectively* dependent on the threshold cluster size ($n_t$) of force onset and the strength ($F$) of pulling; the larger the threshold size, the higher the plateau, i.e., the greater the coverage of Ag in the multifocal pattern; the stronger the force, the wider the plateau, i.e., the higher the affinity required for the percolating phase to take over.

Since the actual size of BCR-Ag clusters as well as the timing and strength of pulling forces still awaits experimental measurements, we consider alternative schemes of force application and show that qualitative results remain unchanged. An interesting finding is that the scheme we presented in the main text, i.e., pulling on clusters above a modest size with force magnitude that scales with the cluster size, seems to be a favorable scheme, both in regard to energy cost and discriminative ability, compared to the alternatives.

### A. Varying the threshold cluster size

We have assumed that normal pulling forces act only on BCR clusters greater than a threshold size $n_t$. Rather than emphasizing the actual number of this threshold, which is yet to be determined potentially by force measurement combined with single-molecule tracking experiment [1, 3], we suggest that the typical size should be greater than one but relatively small compared to the total number of bound complexes that would form in the absence of pulling.

Fig. S4 shows that, multifocal patterns are robust to change in $n_t$ as long as $n_t > 1$, and the typical cluster size peaks around $n_t$ (Fig. 3c for $n_t = 20$; Fig. S5 for $n_t = 200$). For $n_t = 1$ (blue curve in Fig. S4), the plateau regime disappears, because the collective effect of pulling is lost; this results in an absence of discrimination for moderate affinities. Once finite attachments occur at sufficiently strong affinities, the system will proceed to complete phase separation. Thus, multifocal patterns do not form if every single bond is pulled. Accordingly, the fact that multifocal patterns do form in maturing B cells might suggest that pulling forces indeed act on finite-size clusters rather than single BCR-Ag complexes.

At the other extreme, for very large $n_t$ ($n_t = 200$, red curve in Fig. S4), a high and flat plateau indicates suboptimal discrimination; very few near-threshold clusters persist, insensitive to affinity change. At a finite yet modest threshold size (e.g. $n_t = 20$, green curve in Fig. S4), however, change in Ag coverage tracks variation in affinity over a wide range.

In sum, a moderate level of clustering prior to pulling would allow B cells to benefit from the collective nature of mechanical regulation of the contact pattern (i.e., tuning the size and number of Ag clusters) and thereby achieve discrimination over a broader affinity range than what is possible on the single-molecule level ($n_t = 1$) or under complete phase separation ($n_t$ being comparable to no-force Ag coverage).

Also note that the coarsening transition, $U^*_{BA}$, where the discrimination curves first depart from the plateau (for $n_t > 1$) or from zero attachment (for $n_t = 1$), is independent of $n_t$ (Fig. S4, $U^*_{BA} \simeq 9k_BT$ in all cases), as predicted by the phenomenological model (Eq. 7, SI section II).

### B. Fixed total force on each above-threshold cluster

If we consider a load-sharing scenario in which the total force on each of the above-threshold clusters is independent of the cluster size and constant in time, the discrimination curves only change in quantitative ways, as described below and shown in Fig. S6.

First, multifocal patterns can still form in this load-sharing setting (see cluster size distribution in Fig. S7), but it requires much stronger total forces acting on the clusters to halt phase separation (red curve in Fig. S6; Movie e), compared to when total force scales with cluster size (Fig. 2 in the main text). This is because when the total magnitude of force on each cluster, $F_t$, is fixed, even if *on average* it is sufficient to prevent clusters from exceeding the threshold size $n_t$, occasionally, large fluctuations in bond count among clusters make some of them well above average and thus resistant to stress; eventually these clusters grow so big to overtake the multifocal pattern (green curve in Fig. S6; Movie f) and form a steady state which resembles the one in the force-free case. Thus, load sharing appears to represent an energetically unfavorable scenario in which the fixed force magnitude $F_t$, if sufficient to hold the biggest clusters below $n_t$, would be wastefully large for constraining the smaller clusters. In contrast, pulling force that adjusts to the cluster size could yield persistent multifocal patterns at reduced energy cost.

Secondly, the "percolating regime" (regime III, main text) occurs in a narrower range of affinities in the case of load sharing, which manifests as a steeper slope rising from the plateau toward the no-force value (red curve in Fig. S6), thus reducing the discernible range of affinity, i.e., discrimination capacity, compared to when total force scales with cluster size.

## IV. REMARKS ON DISCRIMINATION ABILITY

Our model also predicts that best discrimination occurs at intermediate Ag concentrations, where synapses remain broadly selective above a stringent affinity threshold (Fig. S8). Either a deficit or an excess of Ag would reduce the diversity and range of patterning response under force, diminishing the discriminative ability. Detailed model aspects will be presented elsewhere [4]. Also of interest are the transient nature of pulling forces [5] and the effect of multivalency [6, 7] under stress.

Within the developed model, we focus on the amount of bound BCR-Ag complexes in the steady state and characterize affinity discrimination ability based on this quantity. This choice is motivated by recent experiment [5] that shows stable Ag clusters in the GC B cell synapses appear to be extracted (i.e., transferred from the Ag-presenting surface to the B cell) at similar times, only after an active centrifugal flow in the B cell pushed the clusters to the edges of the synapses. This suggests that extraction might happen after the formation of multifocal patterns, and thus the extracted Ag would likely be those that remain bound to BCRs in the steady state, prior to being pushed to the synapse periphery. Explicit modeling of Ag extraction and internalization would also require finer knowledge of Ag presentation by the APC and the kinetics of Ag/BCR recycling through endocytosis by the presenting cell/B cell.

We quantify the discrimination capacity (Fig. 4, main text) by the range of discernible affinity, i.e., above the minimum affinity that allows finite attachment and below the maximum affinity prior to saturation (e.g. Ag coverage reaches, respectively, 1% and 95% of the saturation value at the lower and higher ends of this affinity range). Importantly, this affinity range includes the "plateau" in the discrimination curve where multifocal patterns form. In this multifocal regime, a small difference in binding affinity translates into an appreciable change in the number of Ag clusters (Fig. S2 blue curve) while the cluster size is strongly peaked at the threshold size of pulling onset. As seen in the main Fig. 2, the plateau/multifocal regime extends to higher affinity as pulling strengthens, due to a shifted coarsening transition (SI section II). Therefore, such broadening of the multifocal phase in response to normal forces that arrest phase separation is the main reason for the enhanced discrimination capacity under strong pulling forces.

In fact, the slope of the discrimination curve – the discernibility – can be elevated through generic biological mechanisms. For instance, adhesion-induced spreading of B cells [8] provides a positive feedback between binding and spreading that can lead to a stronger dependence of Ag coverage on affinity, compared to a fixed contact area as assumed in our current model. This process is force-independent and thus having no influence on the width of the plateau/multifocal regime while making the discernibility more prominent.

Taken together, the *range* of discernible affinity, which crucially depends on the *force-sensitive width* of the multifocal phase, captures the essence of pulling-modulated discrimination capacity and serves as a robust measure which is not affected by force-independent processes that may quantitatively modify the discernibility.


[1] E. Natkanski, W.-Y. Lee, B. Mistry, A. Casal, J. E. Molloy, and P. Tolar, Science **340**, 1587 (2013).

[2] F. Vascotto, D. L. Roux, D. Lankar, G. Faure-Andr, P. Vargas, P. Guermonprez, and A.-M. Lennon-Dumnil, Current Opinion in Immunology **19**, 93 (2007), innate immunity/Antigen processing and recognition.

[3] I. Rey, D. A. Garcia, B. A. Wheatley, W. Song, and A. Upadhyaya, "Biophysical techniques to study b cell activation: Single-molecule imaging and force measurements," in *B Cell Receptor Signaling: Methods and Protocols*, edited by C. Liu (Springer New York, New York, NY, 2018) pp. 51–68.

[4] M. Knežević and S. Wang, in preparation (2018).

[5] C. R. Nowosad, K. M. Spillane, and P. Tolar, Nature Immunology **17**, 870 (2016).

[6] A. S. Perelson and C. DeLisi, Mathematical Biosciences **48**, 71 (1980).

[7] T. Curk, J. Dobnikar, and D. Frenkel, Proceedings of the National Academy of Sciences **114**, 7210 (2017).

[8] S. J. Fleire, J. P. Goldman, Y. R. Carrasco, M. Weber, D. Bray, and F. D. Batista, Science **312**, 738 (2006).

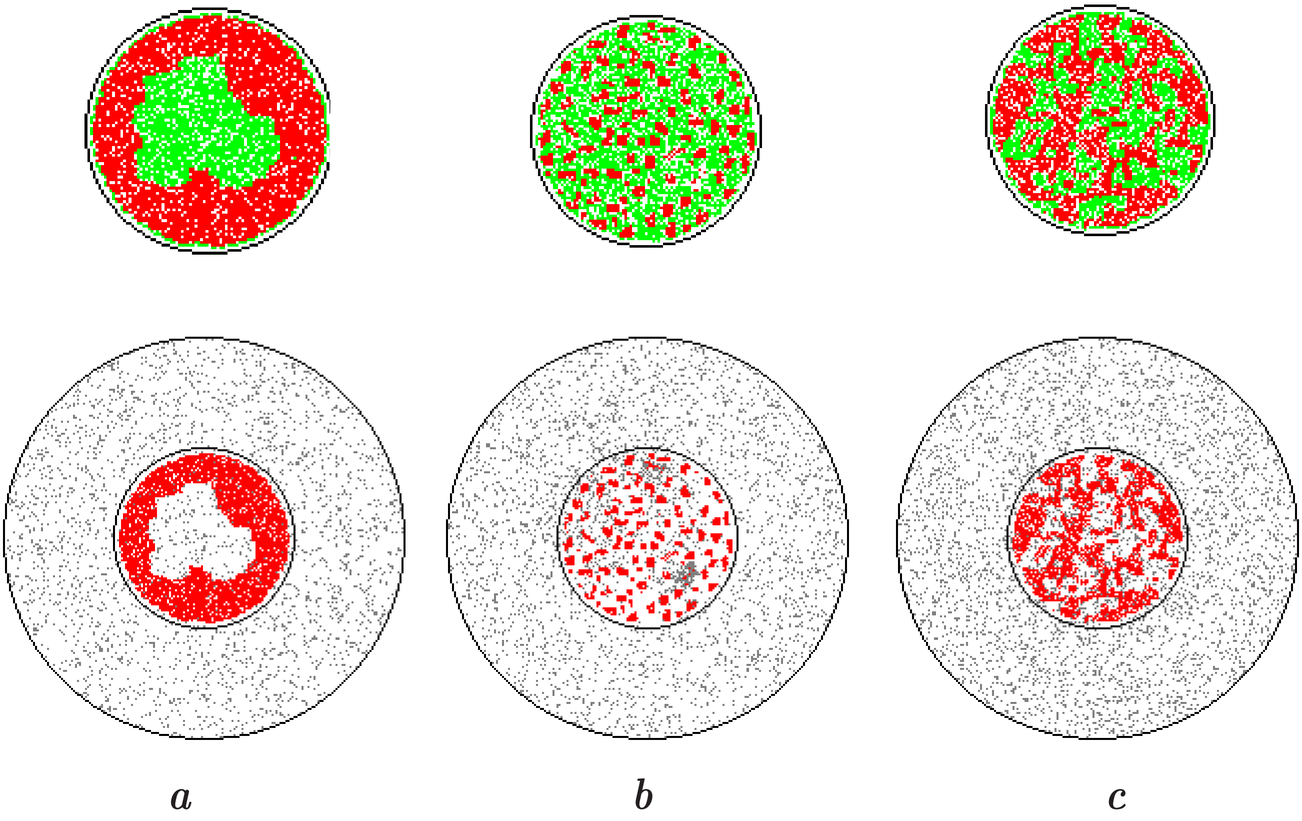


FIG. 1. Pattern formation in B-cell immune synapses: (a) complete phase separation in naive or memory B-cell synapses ($U_{BA} = 6\,k_BT$, $F = 0$), (b) arrested phase separation in maturing B-cell synapses ($U_{BA} = 14\,k_BT$, $Fl = 30\,k_BT$), (c) percolating pattern in maturing B-cell synapses ($U_{BA} = 17\,k_BT$, $Fl = 30\,k_BT$). All other parameters are identical to those in Fig. 2 in the main text. Upper panels show the contact zone; color coding: red – membrane patches with bound BCR-Ag, green – membranes patches with bound adhesion proteins, black – boundary of the contact zone ($r = r_1$), white – all other patches. Lower panels show both the contact and non-adhering zones; color coding: red – membrane patches with BCR-bound Ag, gray – membrane patches with only free Ag molecules, black – boundaries of the circular zones $r = r_1$ and $r = r_2$, white – all other patches. In (a), at lower Ag concentrations, a thinner BCR-Ag ring first forms along the rim of the contact zone but then opens; subsequent relaxation leads to a single compact aggregate in the steady-state pattern.

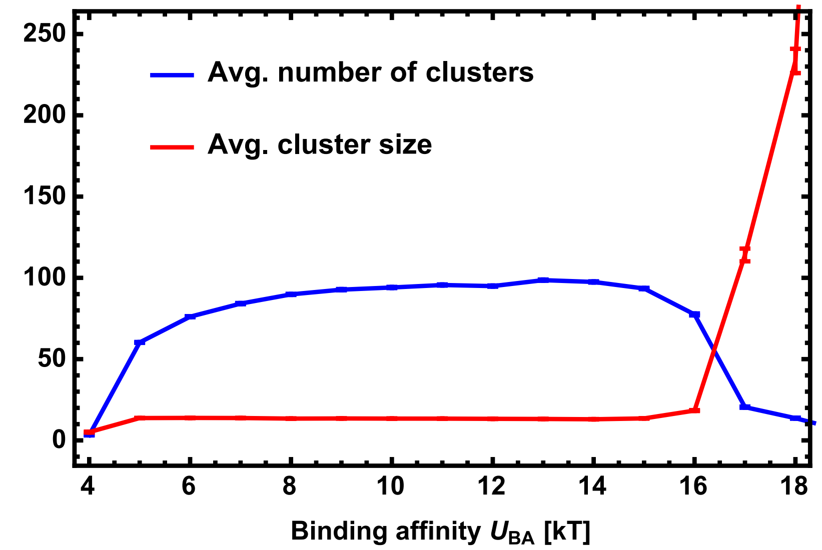


FIG. 2. Statistics of antigen clusters. The average number (blue) and size (red) of antigen clusters formed in the contact zone at large times are shown as a function of BCR-Ag binding affinity $U_{BA}$. Strong pulling forces ($Fl = 30\,k_BT$) are applied to clusters above a threshold size $n_t = 20$. All other parameters are identical to those of Fig. 2 in the main text. The affinity range covers the successive patterning regimes described in the main text, from sparse clusters ($U_{BA} \in [4, 5]\,k_BT$, regime I) to multifocal patterns ($U_{BA} \in [5, 15]\,k_BT$, regime II) to percolating structures ($U_{BA} > 15\,k_BT$, regime III).

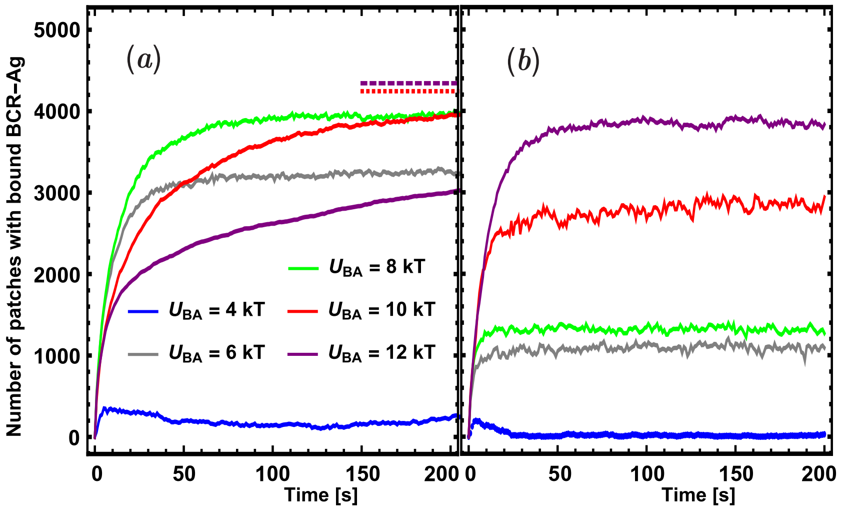


FIG. 3. Efficiency of affinity discrimination. Total number of membrane patches with bound BCR-Ag pairs as a function of time is shown for (a) $F = 0$ and (b) $Fl = 14\,k_BT$ at a series of binding affinities $U_{BA}$ (legends in panel a). The dashed lines in (a) indicate steady-state values for $U_{BA} = 10\,k_BT$ (red) and $U_{BA} = 12\,k_BT$ (purple), which are reached in about 600 s and 4000 s, respectively.

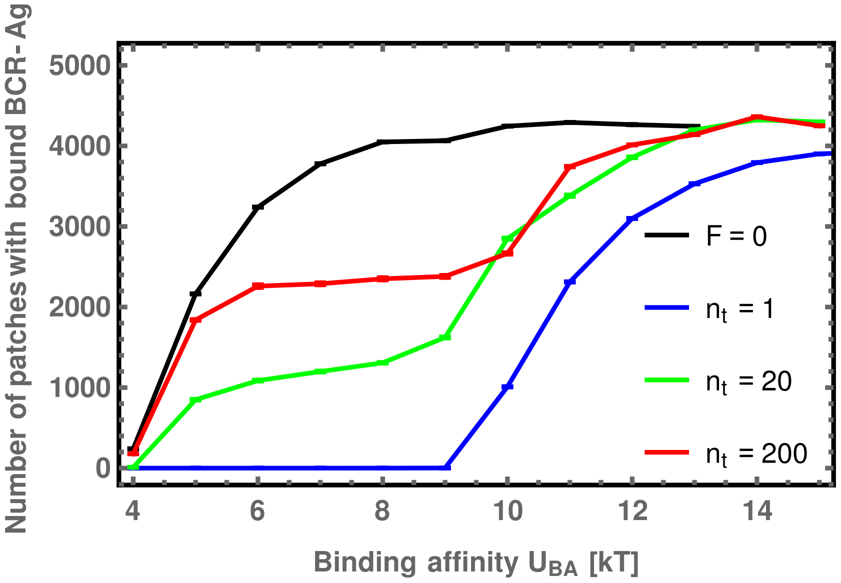


FIG. 4. Affinity discrimination curves at various threshold cluster sizes of pulling onset. When every single BCR-Ag bond is pulled ($n_t = 1$, blue), discrimination is absent for moderate affinities, whereas a very large threshold size ($n_t = 200$, red) yields a high and flat plateau in the multifocal regime and tracing of force-free behavior (black curve) at low affinities. A finite and modest threshold size ($n_t = 20$, green) allows persistent response of Ag coverage to change in affinity over a broad range. The strength of pulling is $Fl = 14k_BT$ in all finite-force cases.

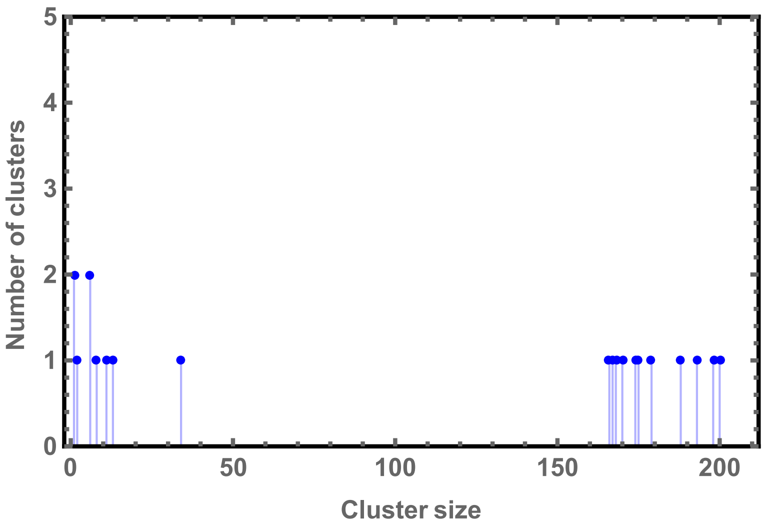


FIG. 5. Distribution of cluster size in the multifocal phase. For a large threshold cluster size ($n_t = 200$) and a moderate affinity ($U_{BA} = 6k_BT$), a small number of near-threshold BCR-bound Ag clusters coexist with a few transient small clusters, resulting in a distinct bimodal distribution. The strength of pulling force is $Fl = 14k_BT$.

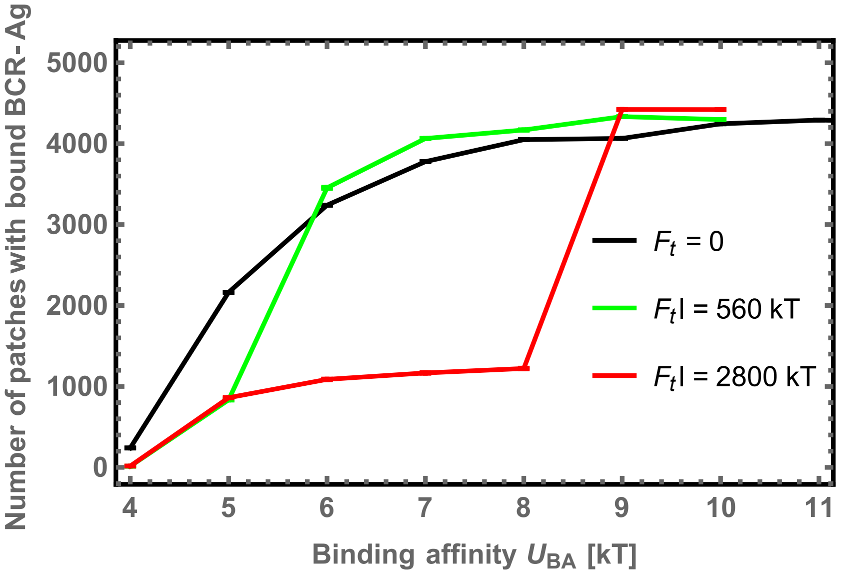


FIG. 6. Affinity discrimination curves in a load-sharing setting. A fixed total force of magnitude $F_t$ applies to each of the above-threshold clusters and distributes evenly among the BCR-Ag bonds. Very strong forces are required to hold the clusters under the threshold size. Red: $F_t l = 2800 k_B T$, multifocal patterns form in the plateau regime; green: $F_t l = 560 k_B T$, no multifocal phase; black: no force. Note for $F_t l = 560 k_B T$, the total force on all clusters combined is comparable to that for $Fl = 14 k_B T$ in the cluster-size-dependent pulling scheme (green curve in Fig. 2, main text). Threshold cluster size of force onset is $n_t = 20$.

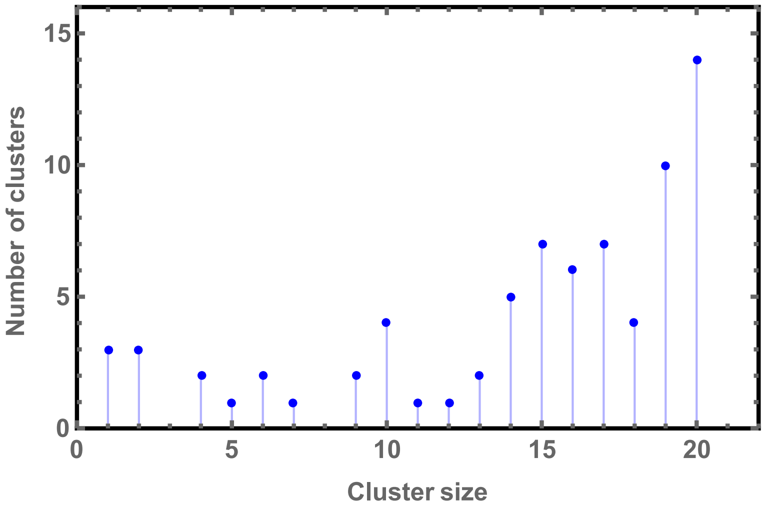


FIG. 7. Distribution of cluster size in the load-sharing scenario. Under very strong pulling forces with a fixed magnitude ($F_t l = 2800 k_B T$) on each of the above-threshold clusters, multifocal patterns form, and the typical cluster size peaks at the threshold size ($n_t = 20$). The binding affinity is moderate ($U_{BA} = 7 k_B T$), insufficient to overcome the disrupting effect of force.

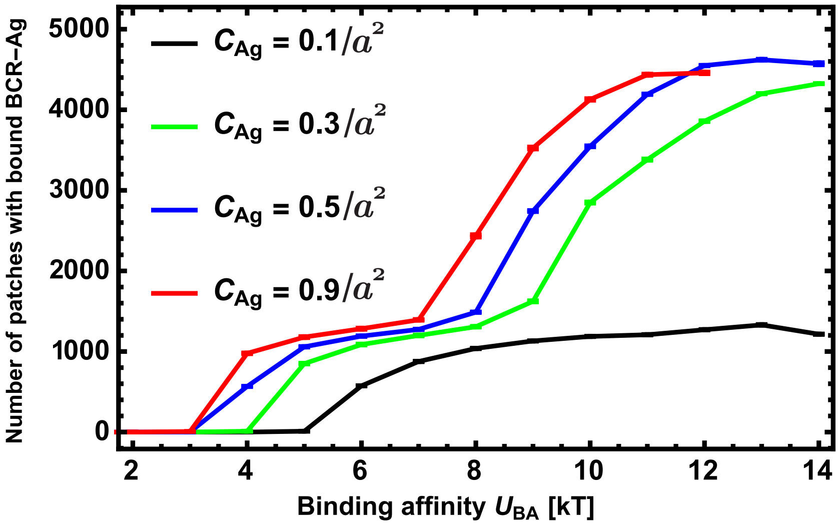


FIG. 8. Affinity discrimination curves at various antigen concentrations. Pulling forces ($Fl = 14\, k_B T$) are applied to clusters above a threshold size $n_t = 20$. Intermediate antigen concentrations (e.g. $C_{Ag} = 0.3/a^2$, green) lead to best discrimination quality and capacity: synapses are broadly selective above a stringent threshold. High concentrations (e.g. $C_{Ag} = 0.9/a^2$, red) lead to saturation of Ag extraction at modest affinities and a low affinity threshold for finite attachments, whereas low concentrations (e.g. $C_{Ag} = 0.1/a^2$, black) leave Ag clusters separate, phase separation arrested, and percolating phase absent.
